# Supplementary material for: Photo-to-Shape Material Transfer for Diverse Structures
Source: arXiv:2205.04018 source file (2022-05-09)
Supplement: Supplementary file 6 [file other.pdf]

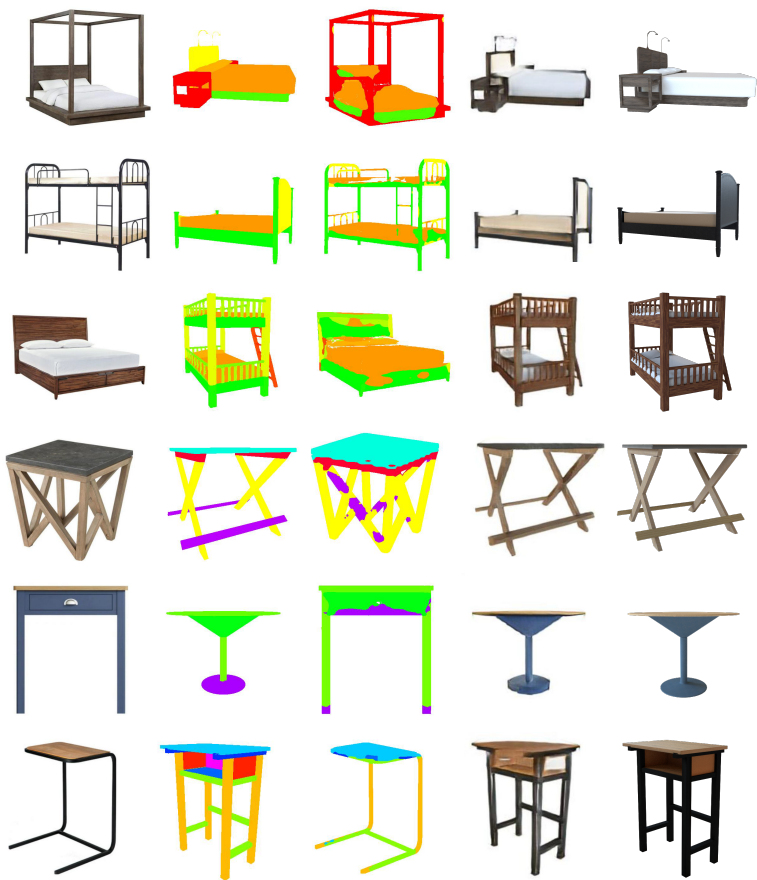
 $P_c$ 
 $O_s$ 
 $\hat{P}_s$ 
 $\hat{O}_c$ 

Result
